# Supplementary material for: Long-term tracking of social structure in groups of rats
Source: arXiv:2408.08945 source file (2024-08-16)

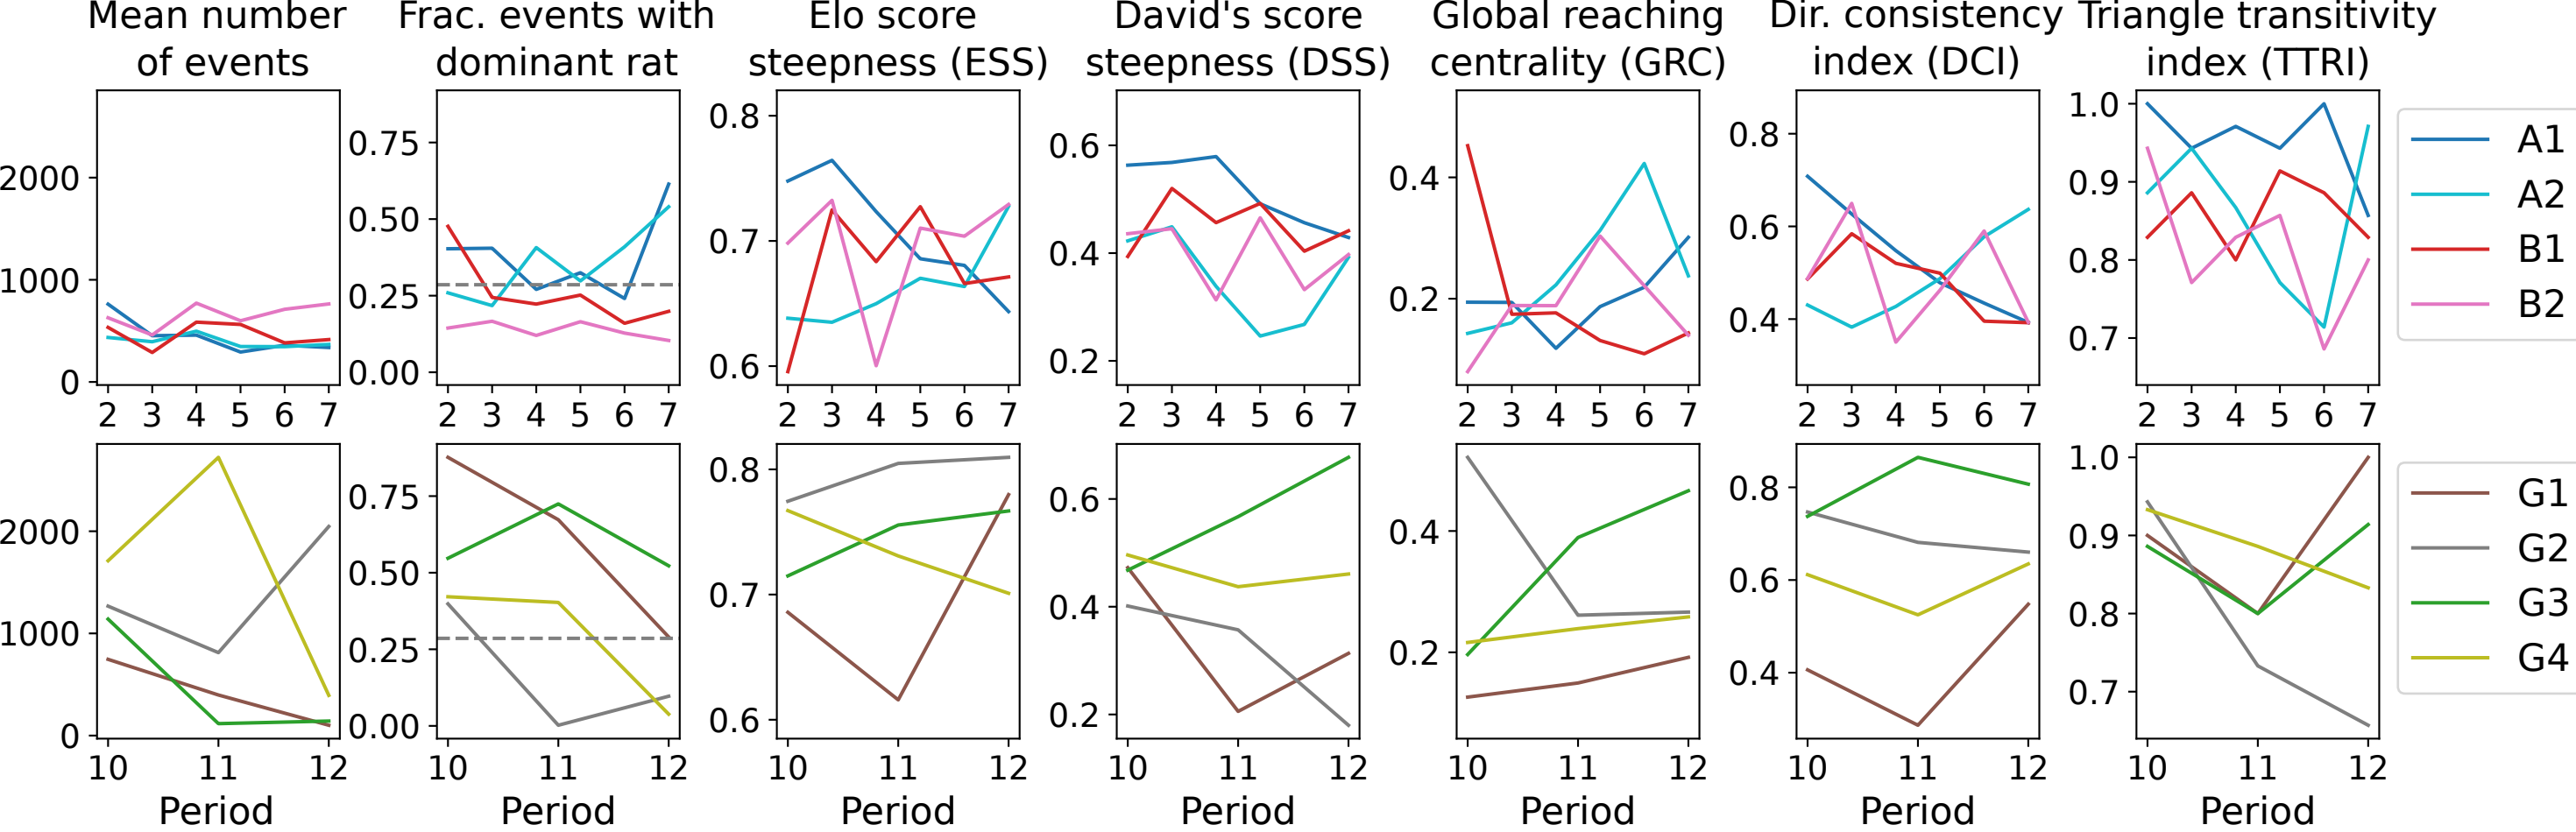

Supplement: Supplementary file 1 [file Supp-networkmetrics-overtime.pdf]
